# Supplementary material for: Sanity Check for External Clustering Validation Benchmarks using Internal Validation Measures
Source: arXiv:2209.10042 source file (2022-09-20)
Supplement: Supplementary file 1 [file A_within_axioms.tex]

\section{Detailed Description of \textit{Within-Dataset} Axioms}

\label{app:within}

% \mac{Put all that material in appendix, keep only one paragraph summarizing the four axioms. Michael: Double-check there is no error in reproducing the definitions and their interpretation. Let us name within-axioms W1, W2... and our new between-axioms B1, B2...}

% The first within-dataset axiom requires the measures to be invariant against the change of scale.

\textbf{(Axiom W1) \textit{Scale Invariance.} } \textit{A measure $f$ satisfies scale invariance if $\forall X$, $ \forall d$, $\forall C$ over $(X, d)$, $f(C, X, d) = f(C, X, \alpha d)$ $\forall \alpha > 0$ (where  $\alpha d$ is a distance function satisfying $\alpha d(x,y) = \alpha \cdot d(x,y)$, $ \forall x, y \in X$) }

% The second axiom asks whether a measure is consistent, which means its value increases when the contrast between within-compactness and between-separability of the classes gets bigger. \

% In other words, $d'$ has smaller within-cluster distance and bigger between-cluster distance compared to $d$ over $C$. Then, the axiom is defined as:

\textbf{$C$-consistent variant.} $d'$ is a $C$-consistent variant of $d$ if $d'(x, y) \leq d(x,y)$ implies $x \sim_C y$, and $d'(x, y) \geq d(x,y)$ implies $ x \nsim_C y$

\textbf{(Axiom W2) \textit{Consistency.} } \textit{A measure $f$ satisfies consistency if  $\forall X$, $ \forall d$, $\forall C$ over $(X, d)$, whenever $d'$ is a $C$-consistent variant of $d$, $f(C, X, d') \geq f(C, X, d)$.}

% The third axiom requires the measures to be rich; any clustering should have an opportunity to have a best score over the domain by modifying the distance function. 

\textbf{(Axiom W3) \textit{Richness. }} \textit{A measure $f$ satisfies richness if $\forall X$, $\forall C$ over $X$, there exists $d$ over $X$ such that $C = \arg\max_{C_i \in \mathcal{C}}f(C_i, X, d)$ (where  $\mathcal{C}$ denotes the set of all possible clusterings over $X$)}

% The last axiom is added to prevent a function that consider the identity of domain points (e.g., relate class labels to the score) to be regarded as a within-dataset internal measure.

\textbf{Clustering Isomorphism. } \textit{Two clustering $C, C'$ over $(X, d)$ are isomorphic (i.e., $C \approx_d C' $), if there exists distance-preserving isomorphism $\phi: X \rightarrow X$, such that $\forall x, y \in X$, $x \sim_C y$ if and only if $\phi(x) \sim_{C'} \phi(y)$.} 

\textbf{(Axiom W4) \textit{Isomorphism Invariance}.} \textit{A measure $f$ satisfies isomorphism invariance if $\forall X$, $ \forall d$, $\forall C, C'$ where $C \approx_d C'$, $f(C, X, d) = f(C', X, d)$. }
