# Supplementary material for: Sanity Check for External Clustering Validation Benchmarks using Internal Validation Measures
Source: arXiv:2209.10042 source file (2022-09-20)
Supplement: Supplementary file 2 [file B_theorem_proof.tex]

\section{Theorems and Proofs}

\subsection{About Calinski-Harabasz Index ($CH$) and Axioms}

% \mac{CH index is not mention in Miligan paper which is cited in BenDavid for studying techniques that all verify Within datasets axioms. So here we prove that CH verify the within-datasets axioms. Therefore CHbtwn also verify these axioms.}

\textbf{Theorem 1.} \textit{Calinski-Harabasz Index ($CH$) satisfies Scale Invariance.}

\textit{Proof. } Consider $C$ over $(X, d)$, and assume that $d'$ be a distance function satisfying $d' = \alpha d(x,y)$ for $\alpha > 0$. Then, 
\[
CH(C, X, d') =  \frac{\sum_{i=1}^{|C|}|C_i|\alpha^2 d^2(c_i, c) / (|C| - 1)}{\sum_{i=1}^{|C|} \sum_{x \in C_i} \alpha^2  d^2(x, c_i) / (|X| - |C|)} = \frac{ \alpha ^2}{\alpha^2 } CH(C, X, d) = CH(C, X, d).
\]
Therefore, $CH$ is scale-invariant. \hfill $\Box$

% \textbf{Theorem 2.} \textit{$CH$ satisfies Consistency.}

% \textit{Proof. } Consider $C$ over $(X, d)$, and assume that $d'$ is a $C$-consistent variant of $d$. 

% For denominator, $\sum_{x\in C_i} d^2(x, c_i) = \frac{1}{|C_i|} \sum_{(x, y) \in C_i} d^2(x,y) $  \cite{apostol03amm} (equation 6'). As $d'(x,y) \leq d(x,y)$ for $ (x,y) \in C_i$, 
% \[
% \frac{1}{|C_i|} \sum_{(x, y) \in C_i} d'^2(x,y) \leq \frac{1}{|C_i|} \sum_{(x, y) \in C_i} d^2(x,y),
% \]
% and this implies 
% \[
% \sum_{x\in C_i} d'^2(x, c_i) \leq \sum_{x\in C_i} d^2(x, c_i).
% \]

% For numerator, 
% \[
% d^2(c_i, c_j) =  \frac{1}{|C_i|\cdot |C_j|} \sum_{x \in C_i, y \in C_j}d^2(x, y) - \frac{1}{|C_i|^2} \sum_{(x,y) \in C_i} d^2(x,y) - \frac{1}{|C_j|^2} \sum_{(x,y) \in C_j} d^2(x,y)
% \]
% \cite{apostol03amm} (equation 28). As $d'(x,y) \geq d(x,y)$ for $x \sim_C y$ and $d'(x,y) \leq d(x,y)$ for $x \nsim_C y$, $d'^2(c_i, c_j) \geq d^2(c_i, c_j)$.   Since $c$ is also a centroid of $X$,  $d'^2(c_i, c) \geq d^2(c_i, c)$ for all $c_i$. 

% As the denominator of $CH(C, X, d')$ is always smaller than the one of $CH(C, X, d)$ and the numerator of $CH(C, X, d')$ is always bigger than the one of $CH(C, X, d)$, $CH(C, X, d') \geq CH(C, X, d)$. Therefore, $CH$ is consistent.

\textbf{Theorem 2.} \textit{$CH$ satisfies Richness.}

\textit{Proof. } Let $C$ be a clustering over $X$. Consider $d$ in which satisfies four conditions: (1) $d(c_i,c)=10$ where $c_i$ is a centroid of a cluster within $C$ (2) $d(c'_i,c)=1$ where $c'_i$ is a centroid of a cluster within any other possible clusterings except $C$ (3) $d(x, c_i)=1$ where $c_i$ is a centroid of a cluster within $C$ and $x$ is a member of that cluster (4) $d(x', c'_i)=10$ where $c'_i$ is a cluster within any other possible clusterings except $C$ and $x'$ is a member of that cluster. Then, $C = \arg\max_{C \in \mathcal{C}} f(C, X, d)$ where $\mathcal{C}$ is a set of all possible clusterings. \hfill $\Box$

\textbf{Theorem 3.} \textit{$CH$ satisfies Isomorphism Invariance. }

\textit{Proof. } $CH$ only considers the distances between data points, and does not regards their external identities. Therefore, for two isomorphic clustering ($C \approx_d C')$, $CH(C,X,d) = CH(C', X, d)$. \hfill $\Box$

\textbf{Theorem 4}. \textit{$CH$ does not satisfy Shift Invariance. }

\textit{Proof. } 
Consider a clustering $C$ over $(X, d)$. Then, as 
\[
CH(C, X, d + \beta) = \frac{\sum_{i=1}^{|C|}|C_i|(d(c_i, c) + \beta)^2 / (|C| - 1)}{\sum_{i=1}^{|C|} \sum_{x \in C_i} (d(x, c_i)+\beta)^2 / (|X| - |C|)} \neq CH(C, X, d),
\]
$CH$ does not satisfy Shift Invariance.
\hfill $\Box$

\textbf{Theorem 5}. \textit{$CH$ does not satisfy Class-Cardinality Invariance.}

\textit{Proof.} $CH$ handles entire clusters within $C$ at once, rather than handling them in pairwise. Therefore, $CH$ does not satisfy Class-Cardinality Invariance.    \hfill $\Box$

\textbf{Theorem 6.} \textit{$CH$ does not satisfy Range Invariance.}

\textit{Proof. } The range of $CH$ is $(0, +\infty)$. Therefore, $CH$ is not range invariant.  \hfill $\Box$

\subsection{About Class-Cardinality Invariance}

Ackerman and Ben-David \cite{bendavid08nips} showed that if a function $f'$ satisfies within-dataset axioms, then its aggregation $f(C, X, d)  = \text{agg}_{S \subseteq C, |S = 2|} f'(S, X, d)$ also satisfies the axioms. 

\textbf{Theorem 7.} \textit{If $f'$ satisfies a within-dataset axiom, then $f(C, X, d)  = \text{agg}_{S \subseteq C, |S = 2|} f'(S, X, d)$ also satisfies the axiom.} \cite{bendavid08nips}

Here, we provide a proof for between-dataset axioms. 

\textbf{Theorem 8.} \textit{If $f'$ satisfies Data-Cardinality Invariance, then $f(C, X, d)  = \text{agg}_{S \subseteq C, |S = 2|} f'(S, X, d)$ is also Data-Cardinality Invariance.}

\textit{Proof.} $f(C, X, d) = \text{agg}_{S \subseteq C, |S = 2|} f'(S, X, d) = \text{agg}_{S \subseteq C, |S = 2|} f'(\underline{S}_\alpha, \underline{X}_\alpha, d) = f(\underline{C}_\alpha, \underline{X}_\alpha, d)$. Thus, $f$ satisfies Data-Cardinality Invariance. \hfill $\Box$

\textbf{Theorem 9.} \textit{If $f'$ satisfies Shift Invariance, then $f(C, X, d)  = \text{agg}_{S \subseteq C, |S = 2|} f'(S, X, d)$ is also Shift Invariance.}

\textit{Proof.} $f(C, X, d) = \text{agg}_{S \subseteq C, |S = 2|} f'(S, X, d) = \text{agg}_{S \subseteq C, |S = 2|} f'(S, X, d + \beta) = f(C, X, d + \beta)$. Thus, $f$ satisfies Shift Invariance. 

\textbf{Theorem 10.} \textit{If $f'$ satisfies Range Invariance, then $f(C, X, d)  = \text{agg}_{S \subseteq C, |S = 2|} f'(S, X, d)$ is also Range Invariance.}

\textit{Proof.} $\min_C f'(C, X, d) = 0$ implies $\min_C f(C, X, d) = \min_C \text{agg}_{S \subseteq C, |S = 2|} f'(S, X, d) = 0$. In the same way, $\max_C f'(C, X, d) = 1$ implies $\max_C f(C,X, d) = 1$. Thus, $f$ is Range Invariance.

\subsection{About Between-Dataset Calinski-Harabasz Index ($CH_{btwn}$) and Axioms}

\textbf{Theorem 11.} \textit{$CH_{btwn}$ satisfies Class-Cardinality Invariance.}

\textit{Proof.} By definition, $CH_{btwn}$ is an aggregation of $CH_3$. \hfill $\Box$

\textbf{Theorem 12.} \textit{$CH_{btwn}$ satisfies Scale Invariance.}

\textit{Proof. } Consider $C$ over $(X, d)$.
\begin{multline*}
    CH_1(C, X, \alpha d ) = 
\frac{\sum_{i=1}^{|C|}|C_i|e^{(\alpha \cdot d(c_i, c)) / \sigma_{\alpha d}} / (|C| - 1)}{\sum_{i=1}^{|C|} \sum_{x \in C_i} e^{(\alpha \cdot d(x, c_i))  / \sigma_{\alpha d }} / (|X| - |C|)} \\ 
= 
\frac{\sum_{i=1}^{|C|}|C_i|e^{(\alpha \cdot d(c_i, c)) / (\alpha \cdot \sigma_{d})} / (|C| - 1)}{\sum_{i=1}^{|C|} \sum_{x \in C_i} e^{(\alpha \cdot d(x, c_i))  / (\alpha \cdot \sigma_{d })} / (|X| - |C|)} = CH_1(C, X, d).
\end{multline*}
Therefore, $CH_1$ is scale invariant, and this makes $CH_2$ and $CH_3$, which are the functions that gets $CH_1$ as input, Scale Invariant. Then, as $CH_{btwn}$ is an aggregation of $CH_3$, due to Theorem 7, $CH_{btwn}$ is Scale Invariant. \hfill $\Box$

% \textbf{Theorem 14.} \textit{$CH_{btwn}$ satisfies Consistency.}

% \textif{Proof.} Consider $C$ over $(X, d)$, and assume that $d'$ is a $C$-consistent variant of $d$. 

% In the proof of Theorem 2, we verified $\sum_$ and $d'^2(c_i, c) \geq d^2(c_i,c)$ 

\textbf{Theorem 13. } \textit{$CH_{btwn}$ satisfies Richness}. 

\textit{Proof.} Consider the same $C, X$, and $d$ with the proof of Theorem 2. In the case, $C = \arg\max_{C \in \mathcal{C}} CH_{btwn}(C, X, d)$ where $\mathcal{C}$ is a set of all possible clusterings. \hfill $\Box$

\textbf{Theorem 14.} \textit{$CH_{btwn}$ satisfies Isomorphism Invariance.} 

\textit{Proof.} As $CH$ is, $CH_{btwn} $ only considers the distances between data points, and does not regards their external identities. Therefore, for two isomorphic clustering ($C \approx_d C')$, $CH_{btwn}(C,X,d) = CH_{btwn}(C', X, d)$. \hfill $\Box$

\textbf{Theorem 15.} \textit{$CH_{btwn}$ satisfies Shift Invariance. }

\textit{Proof.} 
\begin{multline*}
    CH_1(C, X, d + \beta) = 
\frac{\sum_{i=1}^{|C|}|C_i|e^{(d(c_i, c) + \beta) / \sigma_{d + \beta}} / (|C| - 1)}{\sum_{i=1}^{|C|} \sum_{x \in C_i} e^{(d(x, c_i) + \beta) / \sigma_{d + \beta}} / (|X| - |C|)} \\ 
= 
\frac{\sum_{i=1}^{|C|}|C_i|e^{d(c_i, c) / \sigma_{d}} / (|C| - 1)}{\sum_{i=1}^{|C|} \sum_{x \in C_i} e^{d(x, c_i)/ \sigma_{d}} / (|X| - |C|)} \cdot \frac{e^\beta}{e^\beta} = CH_1(C, X, d).
\end{multline*}
Therefore, $CH_1$ is Shift Invariant.
This makes $CH_2$ and $CH_3$, which are functions that gets $CH_1$ as input, Shift Invariant. Then, as $CH_{btwn}$ is an aggregation of $CH_3$, due to Theorem 9, $CH_{btwn}$ is Shift Invariance. \hfill $\Box$

% \textbf{Theorem 1.} \textit{For $N$-dimensional Gaussian distribution $G(0, I)$, the mean of Euclidean distances of vectors randomly sampled from the distribution grows in $O(\sqrt{N})$ while standard deviation stays constant (i.e., grows in $O(1)$).}

% \textit{Proof. } For vectors $x_i \sim G(0, I)$ and $y_i \sim G(0, I)$, $(x_1 - x_2) \sim G(0, \sqrt{2}I)$. Thus, $\| x_1 - x_2 \|^2 / 2 \sim \chi^2_N$, which leads to $\| x_1 - x_2 \| / (\sqrt{2}) \sim \chi_N$. Here, mean $\mu$ and standard deviation $s$ of $\chi_N$ is determined as:
% \[ 
% \mu: \sqrt{2}\frac{\Gamma((N+1)/2)}{\Gamma(N/2)}, s: \sqrt{N - \mu^2} \:\: \cite{abell99ap}.
% \]
% Now, by applying S\'andor's inequality \cite{sandor06rgmia}
% $\sqrt{x} \leq \Gamma(X + 1) / \Gamma(X + 1/2) \leq \sqrt{x+ 1/2}$, which is a stronger version of Gautschi's inequality \cite{kershaw83mc},  we know that $\mu$ satisfies
% \[
% \sqrt{2} \cdot \sqrt{\frac{N-1}{2}} \leq \mu \leq \sqrt{2} \cdot\sqrt{\frac{N}{2}}.
% \]
% As  $\sqrt{(N-1)/2} = O(\sqrt{N})$ and $\sqrt{(N)/2} = O(\sqrt{N})$, $\mu=O(\sqrt{N})$.
% The above inequality also leads to the inequality $0 \leq s = \sqrt{N - \mu^2} \leq 1$, which implies $s = O(1)$.

% Hence, the theorem is true. \hfill $\Box$
