# Supplementary material for: Sanity Check for External Clustering Validation Benchmarks using Internal Validation Measures
Source: arXiv:2209.10042 source file (2022-09-20)
Supplement: Supplementary file 3 [file D_experiment_setting.tex]

\section{Detailed Settings in Between-dataset Rank Correlation Analysis}

\label{app:detail_btw}

\textbf{Classifiers settings. } As aforementioned, for consistency, we exploited the setting of Rodr\'iguez et al. \cite{rodriques18kbs}. The hyperparameters are set as follows:
\begin{itemize}
    \item \textbf{Support Vector Machine} (SVM): We used C-support vector classification model with default hyperparameter setting provided by \texttt{sklearn} \cite{pedregosa11jmlr}. 
    \item \textbf{$k$-Nearest Neighbor} ($k$NN): We used $k=1$, and for all other parameters, we used default setting of \texttt{sklearn}. \mac{That is not really good use of KNN, several values should be tried}
    \item \textbf{Multilayer Perceptron} (MLP): We used 500 epochs, learning rate of 0.3, and momentum of 0.2. We used single hidden layer, where the size of the hidden layer is determined as the half the sum of dimension and number of classes. All other parameters are set to the default provided by \texttt{sklearn}. 
    \item \textbf{Naive Bayesian networks} (NB): We used default parameter setting provided by \texttt{sklearn}.
    \item \textbf{Random forest} (RF): We used RF classifier consists of 100 trees with max depth of 10. Remaining parameters are set to the default of \texttt{sklearn}.
    \item \textbf{Logistic regression} (LR): We used 100 iterations. All remaining parameters are set to the default of \texttt{sklearn}.
    \item \textbf{Linear discriminant analysis} (LDA): We used least squares solution solver, and all other parameters are set to the default provided by \texttt{sklearn}.
\end{itemize}

We conducted 5-fold cross validation for each classifier, and used a mean value as a final classification score for a dataset. For the ensemble of classifiers, we used the max combination of the classifiers (i.e., chose the highest score among the classifiers).\mac{we miss the end of the story. we rank the scatterplot based on this classification score.}

\mac{For all supervised techniques, there should be a  grid search over the meta-parameters. you shall use Auto-ML or similar package for Python (pick the one with the most technique and the most recent): https://automl.github.io/auto-sklearn/master/ 
https://hyperopt.github.io/hyperopt-sklearn/
https://auto.gluon.ai/stable/tutorials/tabular\_prediction/tabular-quickstart.html
}

\textbf{Settings for computing ground-truth data-CLM.}
We used \texttt{sklearn} implementation for DBSCAN, $K$-Means, Birch, Agglomerative clustering, \texttt{sklearn-extra} implementation for $K$-Medoids, and \texttt{pyclustering} implementation for $X$-Means. For HDBSCAN, we used the implementation of McInnes et al. \cite{mcinnes17oss}. 
To find the best hyperparameter setting for each clustering technique, we used Bayesian optimization \cite{snoek12neurips} implementation provided by Nogueira \cite{nogueira14github}. For each clustering techniques, we performed five random exploration and 25 steps of optimization, which are the defaults of the implementation. 
The bounds of each technique's hyperparameter is set as follows:
\begin{itemize}
    \item \textbf{DBSCAN}
    \begin{itemize}
        \item \texttt{epsilon}: [0.01, 1.0]
        \item \texttt{min\_samples}: [1, 10]
    \end{itemize}
    \item \textbf{HDBSCAN}
    \begin{itemize}
        \item \texttt{epsilon}: [0.01, 1.0]
        \item \texttt{min\_samples}: [1, 10]
        \item \texttt{min\_cluster\_size}: [2, 50]
    \end{itemize}
    \item \textbf{\textit{K}-Means}
    \begin{itemize}
        \item $K$ (numver of clusters): [2, (number of classes of data) $\cdot$ 3]
    \end{itemize}
    \item \textbf{\textit{K}-Medoids}
    \begin{itemize}
        \item $K$: [2, (number of classes of data) $\cdot$ 3]
    \end{itemize}
    \item \textbf{\textit{X}-Means}
    \begin{itemize}
        \item \texttt{kmax}: [2, 50]
        \item \texttt{tolerance}: [0.01, 1.0]
    \end{itemize}
    \item \textbf{Birch}
    \begin{itemize}
        \item \texttt{threshold}: [0.1, 1.0]
        \item \texttt{branching\_factor}: [10, 100]
    \end{itemize}
    \item \textbf{Agglomerative Clustering}
    \begin{itemize}
        \item number of clusters: [2, (number of classes of data) $\cdot$ 3]
    \end{itemize}
\end{itemize}
After finding the best hyperparameter setting of a clustering technique for a given datasets, we ran the technique 20 times with same setting and report the average value as the final score.

\newpage
