# Supplementary material for: Sanity Check for External Clustering Validation Benchmarks using Internal Validation Measures
Source: arXiv:2209.10042 source file (2022-09-20)
Supplement: Supplementary file 4 [file E_datasets.tex]

\section{Datasets used in Rank Correlation Analyses}

\label{app:datasets}

\mac{Add another table (two columns) showing all datasets ranked by their decreasing value of CHbtwn, together with the CHbtwn score}

\begin{table}[H]
    
  \caption{Real-World Datasets used in Between-dataset and Within-Dataset Rank Correlation Analyses }
  \label{dataset-table}
  \centering \small
  \begin{tabular}{lllll}
    \toprule
    Dataset & Objects & Features & Classes & Reference \\
    \midrule
        Birds Bones and Living Habits & 413 & 10 & 6 & Kaggle~\cite{kaggle} \\
        Cardiovascular Study Dataset & 2,927 & 15 & 2 & Kaggle \\
        Credit Risk Classification Dataset & 976 & 11 & 2 & Kaggle \\
        Customer Classification & 1,000 & 11 & 4 & Kaggle \\
        Fraud detection bank dataset 20K records binary & 20,468 & 112 & 2 & Kaggle \\
        Heart Attack Analysis \& Prediction Dataset & 303 & 13 & 2 & Kaggle \\
        League of Legends Diamond Games & 48,651 & 17 & 2 & Kaggle \\
        Microbes Dataset & 30,527 & 24 & 10 & Kaggle \\
        Mobile Price Classification & 2,000 & 20 & 4 & Kaggle \\
        Music Genre Classification & 1,000 & 26 & 10 & Kaggle \\
        Orbit Classification For Prediction / NASA & 1,748 & 11 & 6 & Kaggle \\ % Orbit NASA
        Paris Housing Classification & 10,000 & 17 & 2 & Kaggle \\
        pH-recognition & 653 & 3 & 15 & Kaggle \\
        Rice Seed Dataset (Gonen\&Jasmine) & 18,185 & 10 & 2 & Kaggle \\ % Rice type classification
        Siberian Weather Stats & 1,439 & 11 & 9 & Kaggle \\
        Smoker Condition & 1,012 & 7 & 2 & Kaggle \\
        Water Quality & 2,011 & 9 & 2 & Kaggle \\
        Wine Customer Segmentation & 178 & 13 & 3 & Kaggle \\ % Wine Customer
        
        banknote authentication & 1,372 & 4 & 2 & UCI ML Repo~\cite{asuncion07uci} \\
        Breast Cancer Wisconsin (Prognostic) & 569 & 30 & 2 & UCI ML Repo \\
        Breast Tissue & 106 & 9 & 6 & UCI ML Repo \\
        CNAE-9 & 1,080 & 856 & 9 & UCI ML Repo \\
        Dermatology & 358 & 34 & 6 & UCI ML Repo \\
        Echocardiogram & 61 & 10 & 2 & UCI ML Repo \\
        Ecoli & 336 & 7 & 8 & UCI ML Repo \\
        Glass Identification & 214 & 9 & 6 & UCI ML Repo \\
        Harberman's Survival & 306 & 3 & 2 & UCI ML Repo \\
        Hepatitis & 80 & 19 & 2 & UCI ML Repo \\
        Image Segmentation & 210 & 19 & 7 & UCI ML Repo \\
        Ionosphere & 351 & 34 & 2 & UCI ML Repo \\
        Iris & 150 & 4 & 3 & UCI ML Repo \\
        Letter Recognition & 20,000 & 16 & 26 & UCI ML Repo \\
        MAGIC Gamma Telescope & 19,020 & 10 & 2 & UCI ML Repo \\
        Optical Recognition of Handwritten Digits & 3,823 & 64 & 10 & UCI ML Repo \\
        Pen-Based Recognition of Handwritten Digits & 7,494 & 16 & 10 & UCI ML Repo \\
        Planning Relax & 182 & 12 & 2 & UCI ML Repo \\
        SECOM & 1,567 & 590 & 2 & UCI ML Repo \\ % secom
        Spambase & 4,601 & 57 & 2 & UCI ML Repo \\
        SPECTF Heart & 80 & 44 & 2 & UCI ML Repo \\
        Statlog (German Credit Data) & 1,000 & 24 & 2 & UCI ML Repo \\ % German Credit Numeric
        Statlog (Image Segmentation) & 2,310 & 19 & 7 & UCI ML Repo \\
        Taiwanese Bankruptcy Prediction Data Set & 6,819 & 95 & 2 & UCI ML Repo \\ % Company Bankruptcy Prediction
        Wine & 178 & 13 & 3 & UCI ML Repo \\
        Yeast & 1,484 & 8 & 10 & UCI ML Repo \\
        Zoo & 101 & 16 & 7 & UCI ML Repo \\
        
        Blood Transfusion Service Center & 748 & 4 & 2 & Yeh et al.~\cite{yeh2009knowledge} \\
        Boston & 154 & 13 & 3 & Sedlmair et al.~\cite{sedlmair2012taxonomy} \\
        Breast Cancer Coimbra & 116 & 9 & 2 & Patrício et al.~\cite{patricio2018using} \\
        Breast Cancer Wisconsin (Original) & 683 & 9 & 2 & Wolberg et al.~\cite{wolberg1990multisurface} \\
        CIFAR10 & 3,250 & 1,024 & 10 & Krizhevsky et al.~\cite{krizhevsky2009learning} \\ % cifar10
        Classification in asteroseismology & 1,001 & 3 & 2 & Hon et al.~\cite{hon2017deep} \\
        COIL20 & 1,440 & 400 & 20 & Nene et al.~\cite{nene20columbia} \\ % coil20
        Crowdsourced Mapping & 10,545 & 28 & 6 & Johnson et al.~\cite{johnson2016integrating} \\
        Date Fruit Datasets & 898 & 34 & 7 & Koklu et al.~\cite{koklu2021classification} \\
        Diabetic Retinopathy Debrecen Data Set & 1,151 & 19 & 2 & Antal et al.~\cite{antal2014ensemble} \\
        Dry Bean Dataset & 13,611 & 16 & 7 & Koklu et al.~\cite{koklu2020multiclass} \\
        Durum Wheat Features & 9,000 & 236 & 3 & Kaya et al.~\cite{kaya2019towards} \\
    \bottomrule
    
  \end{tabular}
  
\end{table}

\begin{table}[H]
  \label{dataset-table2}
  \centering \small
  \begin{tabular}{lllll}
    \toprule
    Dataset & Objects & Features & Classes & Reference \\
    \midrule
        Epileptic Seizure Recognition & 5,750 & 178 & 5 & Andrzejak et al.~\cite{andrzejak2001indications} \\ % epileptic
        ExtyaleB & 319 & 30 & 5 & Georghiades et al.~\cite{georghiades2001few} \\
        Fashion-MNIST & 3,000 & 784 & 10 & Xiao et al.~\cite{xiao2017fashion} \\ % fashion mnist
        Fetal Health Classification & 2,126 & 21 & 3 & Ayres-de-Campos et al.~\cite{ayres2000sisporto} \\
        Flickr Material Database & 997 & 1,536 & 10 & Sharan et al.~\cite{sharan2009material} \\ % fmd
        HAR & 735 & 561 & 6 & Anguita et al.~\cite{anguita2012human} \\ % har
        Hate Speech & 3,221 & 100 & 3 & Davidson et al.~\cite{davidson2017automated} \\ % hatespeech
        Heart Disease & 297 & 13 & 5 & Detrano et al.~\cite{detrano1989international} \\
        HIVA & 3,076 & 1,617 & 2 & Guyon et al.~\cite{guyon2007agnostic} \\ % hiva
        HTRU2 & 17,898 & 8 & 2 & Lyon et al.~\cite{lyon2016fifty} \\ % Pulsar Dataset HTRU2
        Human Stress Detection & 2,001 & 3 & 3 & Rachakonda et al.~\cite{rachakonda2019stress} \\ % Stress Detection
        IMDB & 3,250 & 700 & 2 & Maas et al.~\cite{maas2011learning} \\ % imdb
        Insurance Company Benchmark  & 5,822 & 85 & 2 & Putten et al.~\cite{van2004bias} \\ % The Insurance Company (TIC) Benchmark
        Labeled Faces in the Wild & 2,200 & 5,828 & 2 & Huang et al.~\cite{huang2008labeled} \\
        Mammographic Mass & 830 & 5 & 2 & Elter et al.~\cite{elter2007prediction} \\
        Mnist64 & 1,082 & 64 & 6 &  Xia et al.~\cite{xia22tvcg} \\
        Olivetti faces dataset & 400 & 4,096 & 40 & AT\&T Lab. Cambridge~\cite{atntlab} \\
        Parkinsons & 195 & 22 & 2 & Little et al.~\cite{little2007exploiting} \\ % Parkinsons Disease Dataset
        Patient Treatment Classification & 4,412 & 10 & 2 & Mujiono Sadikin~\cite{sadikin2020} \\
        Pima Indians Diabetes Database & 768 & 8 & 2 & Smith et al.~\cite{smith1988using} \\
        Pistachio Dataset & 2,148 & 28 & 2 & Ozkan et al.~\cite{ozkan2021classification} \\
        Pumpkin Seeds Dataset & 2,500 & 12 & 2 & Koklu et al.~\cite{koklu2021use} \\
        Raisin Dataset & 900 & 7 & 2 & Cinar et al.~\cite{ccinar2020classification} \\
        Rice Dataset Cammeo and Osmancik & 3,810 & 7 & 2 & Cinar et al.~\cite{cinar2019classification} \\
        seeds & 210 & 7 & 3 & Charytanowicz et al.~\cite{charytanowicz2010complete} \\
        Seismic Bumps & 646 & 24 & 2 & Sikora et al.~\cite{sikora2010application} \\ % seismic
        Sentiment Labeled Sentences & 2,748 & 200 & 2 & Kotzias et al.~\cite{kotzias2015group} \\ % sentiment
        SkillCraft1 Master Table Dataset & 3,338 & 18 & 7 & Thompson et al.~\cite{thompson2013video} \\ % SkillCraft-StarCraft
        SMS Spam Collection & 835 & 500 & 2 & Almeida et al.~\cite{almeida2011contributions} \\ % sms
        Street View House Numbers & 732 & 1,024 & 10 & Netzer et al.~\cite{netzer2011reading} \\ % svhn
        student grade pass or fail & 395 & 29 & 2 & Cortez et al.~\cite{cortez2008using} \\
        Turkish Music Emotion Dataset & 400 & 50 & 4 & Er et al.~\cite{er2019music} \\
        User Knowledge Modeling & 258 & 5 & 4 & Kahraman et al.~\cite{kahraman2013development} \\
        Weather & 365 & 192 & 7 & Ventocilla et al.~\cite{ventocilla2020comparative} \\
        Website Phishing & 1,353 & 9 & 3 & Abdelhamid et al.~\cite{abdelhamid2014phishing} \\
        Wilt & 4,339 & 5 & 2 & Johnson et al.~\cite{johnson2013hybrid} \\
        Wine Quality & 4,898 & 11 & 7 & Cortez et al.~\cite{cortez2009modeling} \\
        Wireless Indoor Localization & 2,000 & 7 & 4 & Rohra et al.~\cite{rohra2017user} \\
        World12d & 150 & 12 & 5 & Sedlmair et al.~\cite{sedlmair2012taxonomy} \\
    \bottomrule
    
  \end{tabular}
  
\end{table}
