# Supplementary material for: Sanity Check for External Clustering Validation Benchmarks using Internal Validation Measures
Source: arXiv:2209.10042 source file (2022-09-20)
Supplement: Supplementary file 5 [file C_basis_dataset.tex]

\section{Basis datasets Used in Validity Analysis}

\label{app:basis}

Following figure depicts a subset of basis dataset consists of two 2D Gaussian distribution used in validity analysis. We diversified the dataset in perspective of dimensionality, scale, number of points, and randomness to verify whether our between-dataset IVM satisfies the axioms.

\begin{figure}[h]
    \centering
    \includegraphics[width=\textwidth]{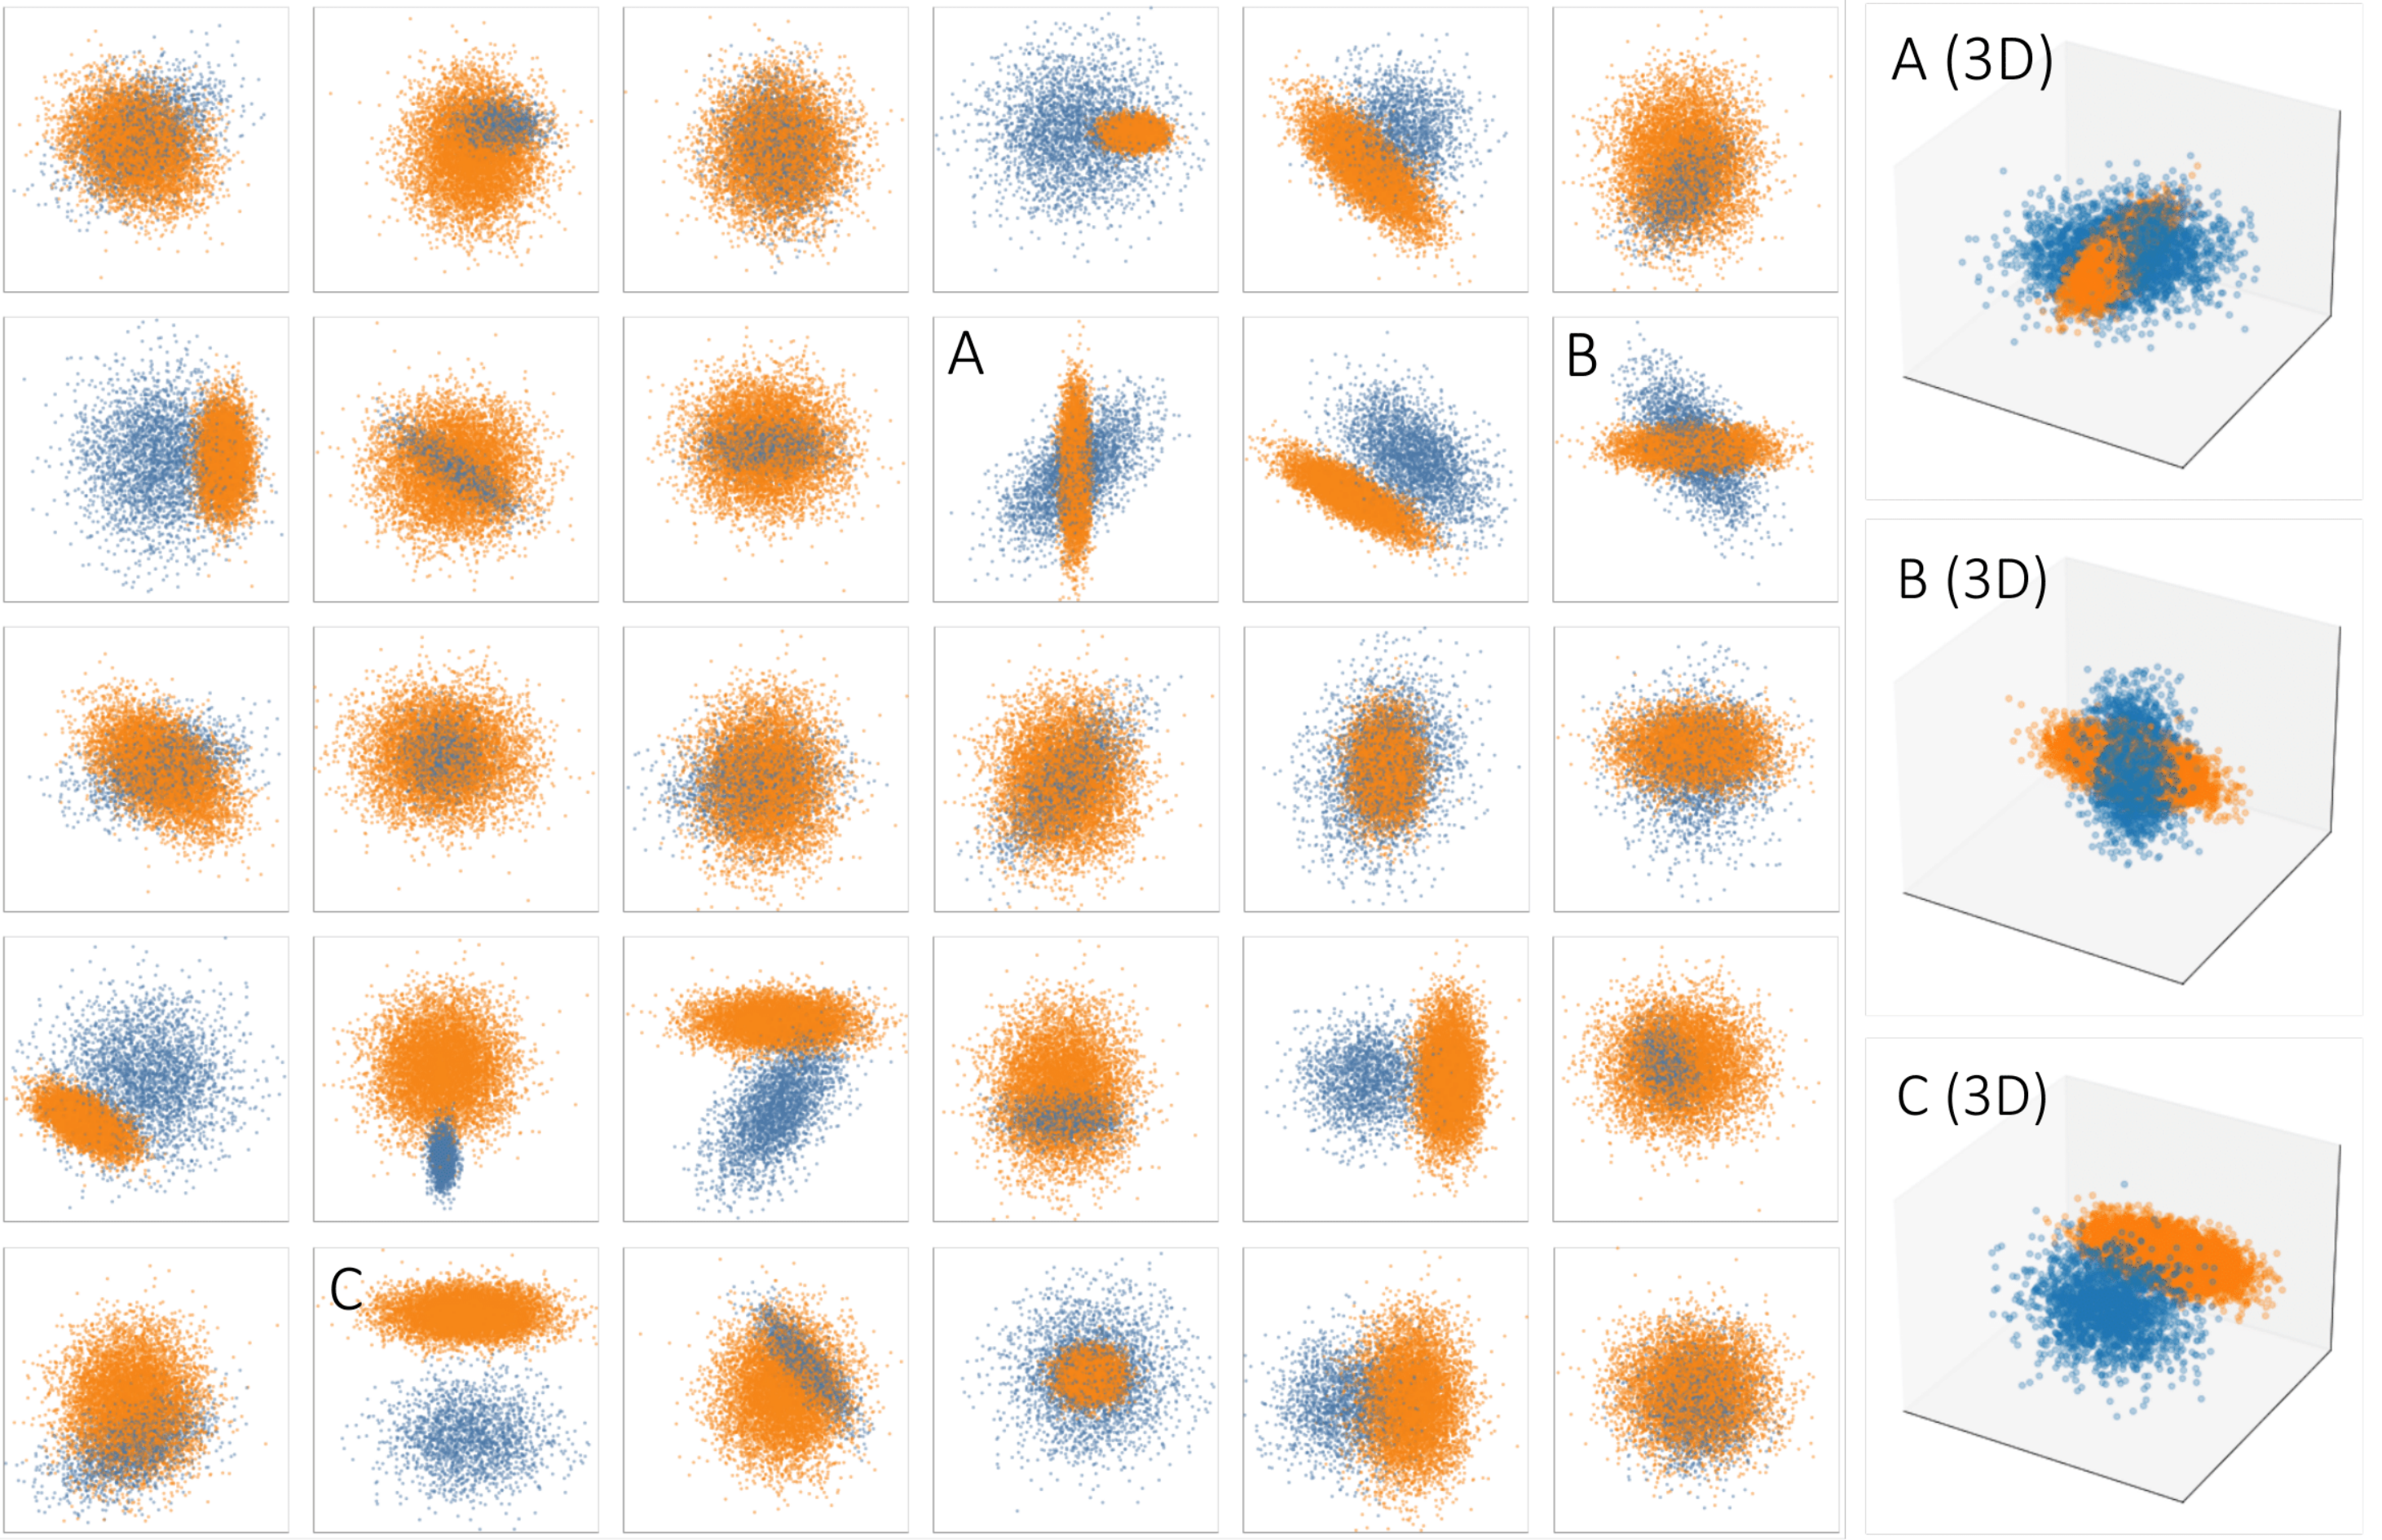} 
    \caption{\mac{Do not use yellow with white background. Use blue/red instead} Subset of 1,000 2D basis datasets used in validity analysis, where each consists of two Gaussian distributions (left) and the dimension-augmented version of the datasets (right). For each 2D dataset, we randomized two distributions' size, variance, and a distance between them. To augment the dimensionality without disturbing the original cluster structure, we added Gaussian noise while maintain the variance of the noise smaller than the original distributions' variance. In this figure, only 3D augmented data was expressed, but data with a higher dimension was also created. }
    \label{fig:validity_data}
\end{figure}
