# Supplementary material for: Sanity Check for External Clustering Validation Benchmarks using Internal Validation Measures
Source: arXiv:2209.10042 source file (2022-09-20)
Supplement: Supplementary file 6 [file F_time_analysis.tex]

\section{Running Time Comparison}

\label{app:time}
