# Supplementary material for: Sanity Check for External Clustering Validation Benchmarks using Internal Validation Measures
Source: arXiv:2209.10042 source file (2022-09-20)
Supplement: Supplementary file 7 [file _deprecated_B_internal_measures.tex]

\section{Detailed Explanation of Internal Measures}
\label{app:im}

\subsection{Internal Clustering Validation}
\label{sec:icv}

As clustering algorithm's goal is to maximize distinction between clusters and similarity within a cluster, most internal measures are designed to measure clusterings based on two criteria: separability and compactness \cite{liu10idcm, tan05idm, zhao02cikm, rendon11ac}. While separability denotes the degree to which clusters are apart from other clusters, compactness represents closeness of the points within a cluster. 
Most measures are defined as the \textit{Ratio} (e.g., Calinski-Harabasz \cite{calinski74cis}, Xie-Beni \cite{xie91tpami}), \textit{Difference }(e.g., Silhouette \cite{rousseeuw87jcam}), or \textit{Sum }(e.g., $S\_Dbw$ \cite{halkidi01icdm}, $CVNN$ \cite{liu13tc}) of two criteria. Here, we list nine widely used internal measures surveyed by Liu et al. \cite{liu10idcm} and Xiong and Li. \cite{xiong13cvm}, and and organize them in three categories. In \autoref{sec:clustgen}, we demonstrate how these measures are generalized to clusterness measures. Note that we only considered monotonic measures, where optimal clustering is determined as the one with maximum or minimum score, instead of the shift point (i.e., the elbow) \cite{halkidi01jiis} which requires subjective determination to be judged. Exact definitions of the measures can be found in Table XXX.




\begin{table}
  \caption{Definition of commonly used internal measures (\autoref{sec:icv}) and their characteristics. Note that there is no fixed range for $SD$ and $CVNN$, as their range depends on normalization factors, which are determined based on currently compared clusterings.}
  \label{sample-table}
  \centering \small
  \begin{tabular}{cclcc}
    \toprule
    Type & Symbol & Definition & Optimal & Range \\
    \midrule
     Ratio & $CH$  & $\frac{\sum_i|C_i|d^2(c_i, c) / (NC-1)}{\sum_i \sum_{x\in C_i} d^2(x, c_i) / (|D| - NC)}$  & max & $(0, \infty)$ \\
     Ratio  & $I$  & $(\frac{1}{NC} \cdot \frac{\sum_{x \in D} d(x, c)}{\sum_i \sum_{x \in C_i} d(x, c_i)} \cdot \max_{i, j} d(c_i, c_j)) ^ p$ ($p=2$ for default)   & max & $(0, \infty)$ \\
     Ratio & $D$  &  $\frac{\min_{i,j} \min_{x \in C_i, y \in C_j} d(x, y)}{\max_k \max_{x, y \in C_k} d(x, y)}$ & max & $(0, \infty)$  \\
    Ratio & $XB$ &  $ \frac{\sum_i \sum_{x \in C_i} d^2(x, c_i)}{|D| \cdot \min_{i, j \neq i} d^2(c_i, c_j)}$ & min & $(0,\infty)$ \\
     Ratio & $DB$   & $\frac{1}{NC} \cdot \sum_i \max_{j\neq i}\frac{\sum_{k =\{i, j\}}(\frac{1}{|C_k|}\sum_{x \in C_k} d(x, c_k))}{d(c_i, c_j)} $ & min & $(0, \infty)$  \\
    Sum & $S\_Dbw$  & $Scat + Dens\_bw$ & min & (0, 2)\\
        &           & $Scat = \frac{1}{NC} \sum_i \| \sigma(C_i) \| / \| \sigma(D) \|$ & &  \\
        &           & $Dens\_bw = \frac{1}{NC \cdot (NC-1)} (\sum_{i, j \neq i} \frac{density(u_{ij})}{\max(density(c_i), density(c_j))})$ &  & \\
    Sum  & $SD$ & $\alpha \cdot Scat + Dis$ & min & - \\
       &        & $Dis = \frac{\max_{i, j} d(c_i, c_j)}{\min_{i, j} d(c_i, c_j)} \cdot \sum_i (\sum_j d(c_i, c_j))^{-1}$ & & \\
    Sum & $CVNN$   & $Sep(k) / \max_{NC} + Com / \max_{NC}$ & min & - \\ 
    & & $Sep = \max_i(\frac{1}{|C_i|} \sum_{j=1, 2, \cdots, |C_i|} \frac{q_j}{k}) $ & & \\
    & & $Com = \sum_i(\frac{2}{|C_i| \cdot (|C_i| -1 ) } \sum_{x,y \in C_i} d(x,y))$ & & \\
    Diff  & $SC$ & $\frac{1}{NC} \cdot \sum_i [\frac{1}{|C_i|} \cdot\sum_{x \in C_i} \frac{b(x) - a(x)}{\max(b(x), a(x))}]$ & min & (-1, 1) \\ 
       &  & $a(x) = \frac{1}{|C_i| - 1} \sum_{y \in C_i, y \neq x} d(x, y)$ & & \\ 
       &  & $b(x) = \min_{j \neq i} (\frac{1}{|C_j|} \sum_{y \in C_j} d(x,y))$ & &\\
    \bottomrule
    \addlinespace[0.115cm]
    \multicolumn{5}{l}{
        \footnotesize
        $D$: dataset; $C_i$: $i$-th cluster; $c / c_i$: centroid of dataset / $i$-th cluster; $NC$: number of clusters;  
    } \\
    \multicolumn{5}{l}{
        \footnotesize
         $d(x, y)$: distances between points $x$ and $y$; $v(C)$: varaince vector of $C$; $\| v \| = \sqrt{v^T \cdot v}$;
    } \\
    \multicolumn{5}{l}{
        \footnotesize
         $u_{ij}$: midpoint of $c_i$ and $c_j$; $density(u_{ij}) = \sum_{x \in D} f(x, u_{ij})$, $density(c_i) = \sum_{x \in C_i} f(x, c_i)$;
    } \\ 
    \multicolumn{5}{l}{
        \footnotesize
         $f(x, c) = 0$ if $d(x, c) > \frac{1}{NC} \sqrt{\sum_i\| \sigma(C_i) \|}$ and else 1; $k$: number of considered nearest neighbors
    } \\ 
    \multicolumn{5}{l}{
        \footnotesize
         $q_j$: number of $C_i$'s $j$-th point's nearest neighbors that are not belong to $C_i$
    } \\ 
  \end{tabular}
  
\end{table}



\textit{Ratio. } 
Calinski-Harabasz index ($CH$) \cite{calinski74cis} evaluates compactness as a sum of squared distances each each point to its cluster centroid, and separability as a sum of squared distances of each cluster centroids to the global centroid of entire dataset. 
I Index ($I$) \cite{maulik02tpami} computes compactness as a ratio of sum of distances of points to its cluster centroid to the sum of points to the global centroid. Separability is defined as a sum of pairwise distances between centroids. 
In Dunn's index ($D$) \cite{dunn74joc}, compactness is  maximum intra-cluster distance and separability is minimum inter-cluster distance. 
Xie-Beni Index ($XB$) \cite{xie91tpami} uses same definition for compactness with $CH$, while defining separability as minimum pairwise distances between centroids.
For Davies-Bouldin Index ($DB$), the similarity of two clusters are first defined where compactness is a sum of distances of points to their cluster centroid, and separability is a distance between centroids. Then, final score is computed as an average of the score assigned to each cluster; each cluster's score corresponds to the max similarity with among the ones with other clusters. 
These measures are defined in a form of $Score = (a \cdot Separability) / (b \cdot Compactness)$ ($CH$, $I$, $D$) or its inverse ($XB$, $DB$). While the higher value implies better clustering in the former, lower value implies better clustering in the latter. 

\textit{Summation. }
S\_Dbw Index ($S\_Dbw$) \cite{halkidi01icdm} evaluates compactness as a ratio of the average of cluster variance to the entire variance of the dataset. Separability instead takes the concept of density; for each pair of clusters, separation is defined as a ratio of density around midpoint of the cluster centroid to the density around centroids. SD Index ($SD$) \cite{halkidi00pkdd}  shares the definition of compactness with $S\_Dbw$, while utilizes the sum of cluster centroids to represent separation. Clustering Validation index based on Nearest Neighbors ($CVNN$)  \cite{liu13tc} compute separability as an average ratio of each points' nearest neighbors belonging to the same cluster to the total number of nearest neighbors. Compactness is computed as an average intra-cluster pairwise distances.
These three measures simply compute the final score as a sum of separability and compactness. However, as the range of separability and compactness can vary, the measures often requires additional adjustment. For example, in $SD$, additional weighting factor is multiplied to compactness to balance it with separability. In contrast, $CVNN$ normalizes both separability and compactness to the maximum separability and compactness computed among all clusterings that are currently compared. 

\textit{Difference. }
Silhouette coefficient ($SC$) \cite{rousseeuw87jcam} quantifies average difference between mean intra-cluster distance (compactness) and the mean nearest-cluster distance (separability) for every point. The optimal clustering is determined as the one having the max index. 


As internal validation measures are naturally designed to find optimal clustering , most of them cannot be used across datasets. 
However, at least $S$ have been used across dataset; it is widely used to evaluate DR by quantifying the extent to which a cluster structure of the original space are well represented in the embeddings \cite{joia11tvcg, fadel15neurocomp}. Still, this use case is about comparing datasets with identical dimension, number of points and clusters. 
Our generalization instead allows the measure to be used across arbitrary datasets, thus enables various useful application scenarios.
